# Supplementary material for: On the Relation Between Mobile Encounters and Web Traffic Patterns: A Data-driven Study
Source: arXiv:1808.03842 source file (2018-11-05)
Supplement: Supplementary file 1 [file appendix.tex]

%\newpage

%\appendix
\numberwithin{equation}{section}

\section*{Appendices}
%\addcontentsline{toc}{section}{Appendices}
%\renewcommand{\thesubsection}{\arabic{subsection}}
%\renewcommand{\thesection}{\arabic{section}}
\setcounter{section}{0}
lalala
